# Supplementary material for: When is Memorization of Irrelevant Training Data Necessary for High-Accuracy Learning?
Source: arXiv:2012.06421 source file (2021-07-21)
Supplement: Supplementary file 1 [file related_work.tex]

\section{Related Work}
\label{sec:related_work}

\subsection{Main Writing}

\paragraph{Empirical Work on Sample Memorization in Deep Learning.}

\paragraph{Differential Privacy.}

\paragraph{Representation Dimension.}
A line of work closely related to the topics studied here is that of \emph{representation dimension}, which arises in the analysis of the sample complexity of private PAC (and agnostic) learning as defined in \cite{kasiviswanathan2011can}.
For a given concept class $C$, \cite{beimel2010bounds} define an $\epsilon$-representation of $C$ as a class of functions $\mathcal{H}$ which, for every data distribution $D$ and every concept $c\in C$, there is an $h\in\mathcal{H}$ such that $\Pr_{x\sim D}[h(x)\neq c(x)]\le \epsilon$.
Such a representation may be much smaller than the concept class itself (it may be finite even when $C$ is infinite) and can be privately learned with $O(\log |\mathcal{H}|)$ samples.
This notion is generalized in \cite{beimel2019characterizing} to that of a probabilistic representation, where $\mathcal{H}$ is chosen randomly from a set and need only be a representation of $C$ with high probability.
In \cite{beimel2019characterizing} the authors show that this characterizes the sample complexity of pure private learning. 

In \cite{feldman2014sample} the connection between representation and communication is made explicit, since a learning algorithm outputting a hypothesis in $\mathcal{H}$ needs exactly $\log |\mathcal{H}|$ bits to specify which one.
The authors prove the equivalence of the sample complexity of differentially-private learning and the randomized one-way communication complexity of evaluating concepts and prove additional bounds using this equivalence.

In our learning settings the labels may not be a deterministic function of the inputs.
This is a feature of machine learning in practice but places us outside the classical settings of PAC or agnostic learning.
Nevertheless, we can compare the guarantees of private learning with our lower bounds.
Similarly to agnostic learning (and in contrast to the PAC model) the learning algorithms we analyze may output arbitrary messages.
Private PAC learning asks for guarantees for worst-case concepts and distributions.
The lower bounds from representation dimension are of the form: for any private learning algorithm using too few samples, there is a choice of distribution $D$ and concept $c$ such that the algorithm will produce a bad hypothesis with high probability.
We provide a joint meta-distribution over data distributions and (randomized) labeling functions such that any learning algorithm will low mutual information will have high error. 

\paragraph{VC Dimension.}
The Vapnik-Chervonekis (VC) dimension of a concept class $C$ is well-known to characterize the sample complexity of PAC and agnostic learning in the absence of privacy.

\paragraph{Time-Space Tradeoffs for Learning.}
A line of work beginning with Raz \cite{raz2018fast} (see \cite{garg2018extractor} for a more recent summary of results) establishes time-space tradeoffs for learning: problems where any learning algorithm requires either a large memory or a large number of samples.
The prime example is parity learning over $d$ bits, which is shown to require either $\Omega(d^2)$ bits of memory or exponentially many samples.
The straightforward algorithm for parity learning requires $O(d)$ samples, so this result shows that any feasible algorithm must store, up to constant factors, as many bits as are required to store the dataset.

Our work sets a specific number of samples under which learning is feasible and, for that number of samples, establishes an information lower bound on the \emph{output} of the algorithm.
This implies not only a communication lower bound but also one on memory usage: the algorithm must store the output immediately prior to releasing it.
Some of our models exhibit the property that, with additional data, an algorithm can output a substantially smaller model.
These learning tasks might exhibit a time-space tradeoff, although not as dramatic as the requirement of exponentially many samples.
Intuitiviely, the underlying concept in parity learning must be learned ``all at once,'' since for example the learner's belief about the bits in the second half of the string depend heavily on its belief about the bits in the first half.
Our problem instances seem to have the property that they can be learned ``piece-by-piece,'' where the algorithm learns a chunk of bits independently of the rest of the sample.

\paragraph{Tracing Attacks.}

\paragraph{Data Interpolation in Deep Learning.}

\paragraph{Information Bottleneck.}

\subsection{Lists of related work}

\subsection{Prior work on memorization}

\begin{itemize}
    \item Empirical work on memorizing whole samples
    \begin{itemize}
        \item \bibentry{carlini2018secret}
        \item \bibentry{radhakrishnan2019overparameterized}
        \item \bibentry{zhang2019identity}
        \item \bibentry{nagarajan2018theoretical}
    \end{itemize}
    \item Theory and empirical work on interpolation and label fitting 
    \begin{itemize}
        \item \bibentry{feldman2020does}
        \item \bibentry{zhang2016understanding}
        \item \bibentry{liang2019multiple}
        \item Much much more...
        \item Important distinction: ``just'' labels?
    \end{itemize}
    \item Privacy, reconstruction, and tracing
    \begin{itemize}
        \item \bibentry{dinur2003revealing}
        \item "Exposed!" survey of attacks on privacy
        \item Those papers aren't really about leaking of entire data vectors; rather they show how to recover single bits about individuals (either "their data bit" or membership). 
    \end{itemize}
    \item Relevant highlights of learning + information theory
    \begin{itemize}
        \item ``Information bottleneck'' analyzes representation of data points, doesn't directly apply here
        \begin{itemize}
            \item Our work gives a different type of information bottleneck in learning
        \end{itemize}
    \item Raz et al.'s line of work on time-space lower bounds in learning
    \begin{itemize}
        \item Looks at space during learning (as opposed to what's in the final model).
        \item If time permits: connect our results to that setting?
    \end{itemize}
    \item Work on representation dimension {\color{red} think more about what to say here}
        \begin{itemize}
            \item Beimel, Brenner, Kasiviswanathan, Nissim '1x, Beimel-Nissim-Stemmer '13,  Feldman-Xiao 
                        \begin{itemize}
                            \item (Part of nice line of work on private learning)
                        \end{itemize}
            \item Major points:            
            \begin{itemize}
                \item Representation dimension captures space/info complexity of the worst-case distribution (for a given concept class)
                \item If concept class and example distribution are fixed, space bounded by size of a distribution-specific cover. 
            \end{itemize}
            \item Interesting consequence: for intervals and LTF's,  learning from minimal number of sample (=VC dimension) can require a hypothesis of size $\Omega(n H(X))$, where $H(X)$ can be arbitrarily large.
        \end{itemize}
    
        \end{itemize}

\end{itemize}

\subsection{Work used or cited in our technical results}

\begin{itemize}
    \item String Completion
    \begin{itemize}
        \item \bibentry{bar2004sketching}
        \item \bibentry{feldman2014sample}
    \end{itemize}
    \item Gap Hamming
    \begin{itemize}
        \item \bibentry{indyk2003tight}
        \item \bibentry{hadar2019communication}
        \item \bibentry{ankitsemail}
        \item Braverman paper stating problem is open (cited in email to Mark)
        \item \bibentry{ahlswede1976spreading}
    \end{itemize}
    \item OR of Equalities
    \begin{itemize}
        \item \bibentry{saglam2013communication}
    \end{itemize}
    \item General reference
    \begin{itemize}
        \item \bibentry{mitzenmacher2017probability} 
        \item \bibentry{cover1991elements}
        \item \bibentry{roughgarden2015communication}
        \item \bibentry{guruswami2012essential}
    \end{itemize}
\end{itemize}

\subsection{Other Background}

\begin{itemize}
    \item \bibentry{dagan2016trading}
    \item \bibentry{fei2006one}
    \item \bibentry{lake2011one}
\end{itemize}
